# Supplementary material for: Hide or Highlight: Understanding the Impact of Factuality Expression on User Trust
Source: arXiv:2508.07095 ancillary file (2025-08-09)
Supplement: Supplementary file 1 [file Supplemental_434.pdf]

## Supplementary Material (Biography Texts)

### Biography 1: Jesse Foppert

#### (a) Biography Text Using the Transparent Strategy

<Question> Tell me a bio of Jesse Foppert

<AI-generated answer>

Jesse Foppert is a former professional baseball player who was born on July 10, 1980, in San Rafael, California, USA. He attended the University of San Francisco and was drafted by the San Francisco Giants in the second round of the 2001 MLB draft. He made his Major League debut with the Giants in 2003 and played for them until 2005. Foppert then spent time with the Seattle Mariners and the Pittsburgh Pirates before retiring from professional baseball in 2008. Over the course of his career, Foppert had a record of 8-9 with a 5.08 ERA and 128 strikeouts in 123 innings pitched.

<Reference> (the link will open in a new window, so don't worry about leaving this survey)

[https://en.wikipedia.org/wiki/Jesse\\_Foppert](https://en.wikipedia.org/wiki/Jesse_Foppert)

#### (b) Biography Text Using the Attention Strategy

<Question> Tell me a bio of Jesse Foppert

<AI-generated answer>

Jesse Foppert is a former professional baseball player who was born on July 10, 1980, in San Rafael, California, USA. He attended the University of San Francisco and was drafted by the San Francisco Giants in the second round of the 2001 MLB draft. He made his Major League debut with the Giants in 2003 and played for them until 2005. Foppert then spent time with the Seattle Mariners and the Pittsburgh Pirates before retiring from professional baseball in 2008. Over the course of his career, Foppert had a record of 8-9 with a 5.08 ERA and 128 strikeouts in 123 innings pitched.

<Reference> (the link will open in a new window, so don't worry about leaving this survey)

[https://en.wikipedia.org/wiki/Jesse\\_Foppert](https://en.wikipedia.org/wiki/Jesse_Foppert)

#### (c) Biography Text Using the Opaque Strategy

<Question> Tell me a bio of Jesse Foppert

<AI-generated answer>

Jesse Foppert is a former professional baseball player who was born on July 10, 1980, [..]. He attended the University of San Francisco and was drafted by the San Francisco Giants in the second round of the 2001 MLB draft. He made his Major League debut with the Giants in 2003 and played for them until 2005. [..]. Over the course of his career, Foppert had a record of 8-9 [..].

<Reference> (the link will open in a new window, so don't worry about leaving this survey)

[https://en.wikipedia.org/wiki/Jesse\\_Foppert](https://en.wikipedia.org/wiki/Jesse_Foppert)

#### (d) Biography Text Using the Ambiguity Strategy

<Question> Tell me a bio of Jesse Foppert

<AI-generated answer>

Jesse Foppert was a baseball player who was born on July 10, 1980, in the US. He attended the University of San Francisco and was drafted by the San Francisco Giants in the second round of the 2001 MLB draft. He made his Major League debut with the Giants in 2003 and played for them until 2005. Foppert spent a lot of time with other teams before stepping away from professional baseball in the 2000s. Foppert had a record of 8-9.

<Reference> (the link will open in a new window, so don't worry about leaving this survey)

[https://en.wikipedia.org/wiki/Jesse\\_Foppert](https://en.wikipedia.org/wiki/Jesse_Foppert)

#### Biography 2: Frederick Howard Taylor

##### (a) Biography Text Using the Transparent Strategy

<Question> Tell me a bio of Frederick Howard Taylor

<AI-generated answer>

Frederick Howard Taylor (1862-1946) was a British missionary and author **who spent most of his life in China**. He was the son of James Hudson Taylor, the founder of the China Inland Mission (CIM), and followed in his father's footsteps **by dedicating his life to spreading the Christian gospel in China**. **Taylor was born in China while** his parents were missionaries there, **and he spent much of his childhood in the country**. He later returned to China as a missionary himself, **first as a teacher in the CIM's schools and later** as a medical missionary. In addition to his missionary work, **Taylor was also a prolific author**. He wrote several books about his experiences in China, including "Hudson Taylor and the China Inland Mission", a biography of his father, **and "Behind the Ranges: The Life-Changing Story of J.O. Fraser"**, a biography of another CIM missionary. **Taylor's legacy continues today through the work of the CIM, which has evolved into the organization now known as OMF International.**

<Reference> (the link will open in a new window, so don't worry about leaving this survey)

[https://en.wikipedia.org/wiki/Frederick\\_Howard\\_Taylor](https://en.wikipedia.org/wiki/Frederick_Howard_Taylor)

##### (b) Biography Text Using the Attention Strategy

<Question> Tell me a bio of Frederick Howard Taylor

<AI-generated answer>

**Frederick Howard Taylor (1862-1946) was a British missionary and author who spent most of his life in China. He was the son of James Hudson Taylor, the founder of the China Inland Mission (CIM), and followed in his**

**father's footsteps** by dedicating his life to spreading the Christian gospel in China. Taylor was born in China while **his parents were missionaries there**, and he spent much of his childhood in the country. **He later returned to China as a missionary himself**, first as a teacher in the CIM's schools and later **as a medical missionary**. **In addition to his missionary work**, Taylor was also a prolific author. **He wrote several books about his experiences in China**, including "**Hudson Taylor and the China Inland Mission**", a biography of his **father**, and "**Behind the Ranges: The Life-Changing Story of J.O. Fraser**", a biography of another CIM missionary. Taylor's legacy continues today through the work of the CIM, which has evolved into the organization now known as OMF International.

<Reference> (the link will open in a new window, so don't worry about leaving this survey)

[https://en.wikipedia.org/wiki/Frederick\\_Howard\\_Taylor](https://en.wikipedia.org/wiki/Frederick_Howard_Taylor)

#### (c) Biography Text Using the Opaque Strategy

<Question> Tell me a bio of Frederick Howard Taylor

<AI-generated answer>

Frederick Howard Taylor (1862-1946) was a British missionary and author [..]. He was the son of James Hudson Taylor, the founder of the China Inland Mission (CIM), and followed in his father's footsteps [..]. [..] his parents were missionaries there, [..]. He later returned to China as a missionary himself, [..] as a medical missionary. In addition to his missionary work, [..]. He wrote several books about his experiences in China, including "Hudson Taylor and the China Inland Mission", a biography of his father [..].

<Reference> (the link will open in a new window, so don't worry about leaving this survey)

[https://en.wikipedia.org/wiki/Frederick\\_Howard\\_Taylor](https://en.wikipedia.org/wiki/Frederick_Howard_Taylor)

#### (d) Biography Text Using the Ambiguity Strategy

<Question> Tell me a bio of Frederick Howard Taylor

<AI-generated answer>

Frederick Howard Taylor was a missionary who was born in 1862 and died in 1946. He was the son of James Hudson Taylor, the founder of the China Inland Mission (CIM), and followed in his father's footsteps by pursuing a religious mission in China. Taylor spent some of his childhood in China where his parents served as missionaries. He later returned to China as a missionary, serving in various roles, including medical. In addition to his missionary work, Taylor was also an author. He wrote several books about his experiences in China, including several biographies, such as "Hudson Taylor and the China Inland Mission", a biography of his father. Some people believe that Taylor's legacy continues today through the work of an organization that has evolved into one with a different name.

<Reference> (the link will open in a new window, so don't worry about leaving this survey)

[https://en.wikipedia.org/wiki/Frederick\\_Howard\\_Taylor](https://en.wikipedia.org/wiki/Frederick_Howard_Taylor)

#### (a) Biography Text Using the Transparent Strategy

<Question> Tell me a bio of Lewis Nkosi

<AI-generated answer>

Lewis Nkosi (1936-2010) was a South African writer, essayist, and literary critic. He was born in Durban, South Africa and grew up during the era of apartheid. He began his writing career as a journalist, working for various newspapers in South Africa, including The Star and Drum magazine. In 1960, Nkosi was arrested for his involvement in anti-apartheid activism and was subsequently forced to leave South Africa. He spent the next several decades living and working in various countries, including England, Zambia, and the United States. Nkosi is best known for his literary criticism, particularly his work on African literature. He was a regular contributor to various literary magazines and newspapers, including The New York Times and The Guardian. Some of his most notable books include "Home and Exile," "Tasks and Masks," and "Mating Birds." Throughout his career, Nkosi received numerous awards and honors, including the Order of Ikhamanga, one of South Africa's highest civilian honors. He passed away in 2010 at the age of 73.

<Reference> (the link will open in a new window, so don't worry about leaving this survey)

[https://en.wikipedia.org/wiki/Lewis\\_Nkosi](https://en.wikipedia.org/wiki/Lewis_Nkosi)

#### (b) Biography Text Using the Attention Strategy

<Question> Tell me a bio of Lewis Nkosi

<AI-generated answer>

Lewis Nkosi (1936-2010) was a South African writer, essayist, and literary critic. He was born in Durban, South Africa and grew up during the era of apartheid. He began his writing career as a journalist, working for various newspapers in South Africa, including The Star and Drum magazine. In 1960, Nkosi was arrested for his involvement in anti-apartheid activism and was subsequently forced to leave South Africa. He spent the next several decades living and working in various countries, including England, Zambia, and the United States. Nkosi is best known for his literary criticism, particularly his work on African literature. He was a regular contributor to various literary magazines and newspapers, including The New York Times and The Guardian. Some of his most notable books include "Home and Exile," "Tasks and Masks," and "Mating Birds." Throughout his career, Nkosi received numerous awards and honors, including the Order of Ikhamanga, one of South Africa's highest civilian honors. He passed away in 2010 at the age of 73.

<Reference> (the link will open in a new window, so don't worry about leaving this survey)

[https://en.wikipedia.org/wiki/Lewis\\_Nkosi](https://en.wikipedia.org/wiki/Lewis_Nkosi)

#### (c) Biography Text Using the Opaque Strategy

<Question> Tell me a bio of Lewis Nkosi

<AI-generated answer>

Lewis Nkosi (1936-2010) was a South African writer, essayist, and literary critic. He [...] grew up during the era of apartheid. He began his writing career as a journalist, working for various newspapers in South Africa, including [...] Drum magazine. [...], Nkosi [...] was subsequently forced to leave South Africa. He spent the next several decades living and working in various countries, including England, Zambia, and the United States. Nkosi is best known for his literary criticism, particularly his work on African literature. He was a regular contributor to various literary magazines and newspapers, including [...] The Guardian. Some of his most notable books include "Home and Exile," "Tasks and

Masks," and "Mating Birds." Throughout his career, Nkosi received numerous awards and honors, including the Order of Ikhamanga, one of South Africa's highest civilian honors. He passed away in 2010 at the age of 73.

<Reference> (the link will open in a new window, so don't worry about leaving this survey)

[https://en.wikipedia.org/wiki/Lewis\\_Nkosi](https://en.wikipedia.org/wiki/Lewis_Nkosi)

#### (d) Biography Text Using the Ambiguity Strategy

<Question> Tell me a bio of Lewis Nkosi

<AI-generated answer>

Lewis Nkosi (1936-2010) was a South African writer, essayist, and literary critic. He was born in a city in South Africa and grew up during the era of apartheid. He began his writing career as a journalist, working for various newspapers in South Africa, including Drum magazine. Around 1960, due to his connection to certain activities, Nkosi was forced to leave South Africa. He spent the next several decades living and working in various countries, including England, Zambia, and the United States. Nkosi is best known for his literary criticism, particularly his work on African literature. His writing has appeared in various literary magazines and newspapers, including The Guardian. Some of his most notable books include "Home and Exile," "Tasks and Masks," and "Mating Birds." Throughout his career, Nkosi received numerous awards and honors, including the Order of Ikhamanga, one of South Africa's highest civilian honors. He passed away in 2010 at the age of 73.

<Reference> (the link will open in a new window, so don't worry about leaving this survey)

[https://en.wikipedia.org/wiki/Lewis\\_Nkosi](https://en.wikipedia.org/wiki/Lewis_Nkosi)

#### Biography 4: Michael Valpy

##### (a) Biography Text Using the Transparent Strategy

<Question> Tell me a bio of Michael Valpy

<AI-generated answer>

Michael Valpy is a Canadian journalist, author, and academic. He was born in 1944 in Montreal, Quebec, and studied at the University of Toronto, where he earned a Bachelor of Arts degree in 1965 and a Master of Arts degree in 1968. Valpy began his journalism career as a reporter for The Globe and Mail in 1968, and went on to work for several other Canadian news outlets, including The Toronto Star, Maclean's magazine, and CBC Radio. In addition to his work as a journalist, Valpy is also an academic. He has taught at several Canadian universities, including Queen's University, the University of Western Ontario, and Carleton University. He has also been a visiting professor at universities in the United States and the United Kingdom. Valpy has written several books on Canadian politics and society, including "The Age of the Mosaic" and "The Pursuit of Happiness: An Agenda for a Better Society". He has received several awards for his work in journalism, including the Canadian Association of Journalists' Award for Investigative Reporting in 1980 and the Atkinson Fellowship in Public Policy in 1998.

<Reference> (the link will open in a new window, so don't worry about leaving this survey)

[https://en.wikipedia.org/wiki/Michael\\_Valpy](https://en.wikipedia.org/wiki/Michael_Valpy)

#### (b) Biography Text Using the Attention Strategy

<Question> Tell me a bio of Michael Valpy

<AI-generated answer>

Michael Valpy is a Canadian journalist, author, and academic. He was born in 1944 in Montreal, Quebec, and studied at the University of Toronto, where he earned a Bachelor of Arts degree in 1965 and a Master of Arts degree in 1968. Valpy began his journalism career as a reporter for The Globe and Mail in 1968, and went on to work for several other Canadian news outlets, including The Toronto Star, Maclean's magazine, and CBC Radio. In addition to his work as a journalist, Valpy is also an academic. He has taught at several Canadian universities, including Queen's University, the University of Western Ontario, and Carleton University. He has also been a visiting professor at universities in the United States and the United Kingdom. Valpy has written several books on Canadian politics and society, including "The Age of the Mosaic" and "The Pursuit of Happiness: An Agenda for a Better Society". He has received several awards for his work in journalism, including the Canadian Association of Journalists' Award for Investigative Reporting in 1980 and the Atkinson Fellowship in Public Policy in 1998.

<Reference> (the link will open in a new window, so don't worry about leaving this survey)

[https://en.wikipedia.org/wiki/Michael\\_Valpy](https://en.wikipedia.org/wiki/Michael_Valpy)

#### (c) Biography Text Using the Opaque Strategy

<Question> Tell me a bio of Michael Valpy

<AI-generated answer>

Michael Valpy is a Canadian journalist, author, and academic. [...]. Valpy began his journalism career as a reporter [...], and went on to work for several other Canadian news outlets, including The Toronto Star, Maclean's magazine, [...]. In addition to his work as a journalist, Valpy is also an academic. [...]. He has received several awards for his work in journalism, including [...], the Atkinson Fellowship in Public Policy [...].

<Reference> (the link will open in a new window, so don't worry about leaving this survey)

[https://en.wikipedia.org/wiki/Michael\\_Valpy](https://en.wikipedia.org/wiki/Michael_Valpy)

#### (d) Biography Text Using the Ambiguity Strategy

<Question> Tell me a bio of Michael Valpy

<AI-generated answer>

Michael Valpy is a Canadian journalist, author, and academic. He was born in the 1940s in Canada, and studied at universities towards a degree. Valpy began his journalism career as a reporter in the 1960s, and went on to work for several Canadian news outlets, including The Toronto Star and Maclean's magazine. In addition to his work as a journalist, Valpy is also an academic. He has taught at several Canadian universities. He has also visited universities in a few countries. Valpy has written several books about Canada. He has received several awards for his work in journalism, including the Atkinson Fellowship in Public Policy later in his life.

<Reference> (the link will open in a new window, so don't worry about leaving this survey)

[https://en.wikipedia.org/wiki/Michael\\_Valpy](https://en.wikipedia.org/wiki/Michael_Valpy)

## Biography 5: Regina Martínez Pérez

### (a) Biography Text Using the Transparent Strategy

<Question> Tell me a bio of Regina Martínez Pérez

<AI-generated answer>

Regina Martínez Pérez was a Mexican journalist known for her coverage of organized crime and corruption in Mexico. She was born on October 28, 1963, in the state of Veracruz, Mexico, and earned a degree in journalism from the Universidad Veracruzana. Martínez started her career as a journalist in the 1980s, working for various newspapers and eventually becoming a correspondent for the national newspaper *Proceso*. She covered a wide range of topics, including politics, human rights, and organized crime, and was known for her fearless reporting. In 2012, Martínez was found dead in her home in Xalapa, Veracruz. She had been beaten and strangled. Her death was widely believed to be related to her reporting on drug trafficking and corruption in Veracruz, and it sparked outrage and protests from journalists and human rights activists in Mexico and around the world. Martínez's death is a tragic reminder of the dangers faced by journalists in Mexico, where violence and intimidation against the media are all too common. She is remembered as a courageous and dedicated journalist who gave her life in pursuit of the truth.

<Reference> (the link will open in a new window, so don't worry about leaving this survey)

[https://en.wikipedia.org/wiki/Regina\\_Mart%C3%ADnez\\_P%C3%A9rez](https://en.wikipedia.org/wiki/Regina_Mart%C3%ADnez_P%C3%A9rez)

### (b) Biography Text Using the Attention Strategy

<Question> Tell me a bio of Regina Martínez Pérez

<AI-generated answer>

Regina Martínez Pérez was a Mexican journalist known for her coverage of organized crime and corruption in Mexico. She was born on October 28, 1963, in the state of Veracruz, Mexico, and earned a degree in journalism from the Universidad Veracruzana. Martínez started her career as a journalist in the 1980s, working for various newspapers and eventually becoming a correspondent for the national newspaper *Proceso*. She covered a wide range of topics, including politics, human rights, and organized crime, and was known for her fearless reporting. In 2012, Martínez was found dead in her home in Xalapa, Veracruz. She had been beaten and strangled. Her death was widely believed to be related to her reporting on drug trafficking and corruption in Veracruz, and it sparked outrage and protests from journalists and human rights activists in Mexico and around the world. Martínez's death is a tragic reminder of the dangers faced by journalists in Mexico, where violence and intimidation against the media are all too common. She is remembered as a courageous and dedicated journalist who gave her life in pursuit of the truth.

<Reference> (the link will open in a new window, so don't worry about leaving this survey)

[https://en.wikipedia.org/wiki/Regina\\_Mart%C3%ADnez\\_P%C3%A9rez](https://en.wikipedia.org/wiki/Regina_Mart%C3%ADnez_P%C3%A9rez)

### (c) Biography Text Using the Opaque Strategy

<Question> Tell me a bio of Regina Martínez Pérez

**<AI-generated answer>**

Regina Martínez Pérez was a Mexican journalist known for her coverage of organized crime and corruption in Mexico. She was born [...] in the state of Veracruz, Mexico, and earned a degree in journalism from the Universidad Veracruzana. Martínez started her career as a journalist in the 1980s, working for various newspapers and eventually becoming a correspondent for the national newspaper [...]. She covered a wide range of topics, including politics, human rights, and organized crime, [...]. In 2012, Martínez was found dead in her home in Xalapa, Veracruz. She had been beaten and strangled. Her death was widely believed to be related to her reporting on drug trafficking and corruption in Veracruz, [...]. [...]. [...].

**<Reference>** (the link will open in a new window, so don't worry about leaving this survey)

[https://en.wikipedia.org/wiki/Regina\\_Mart%C3%ADnez\\_P%C3%A9rez](https://en.wikipedia.org/wiki/Regina_Mart%C3%ADnez_P%C3%A9rez)

**(d) Biography Text Using the Ambiguity Strategy**

**<Question>** Tell me a bio of Regina Martínez Pérez

**<AI-generated answer>**

Regina Martínez Pérez was a Mexican journalist known for her coverage of organized crime and corruption in Mexico. She was born in 1963, in the state of Veracruz, Mexico, and earned a degree in journalism from the Universidad Veracruzana. Martínez started her career as a journalist in the 1980s, working for various newspapers and eventually becoming a correspondent for a national newspaper. She covered a wide range of topics, including politics, human rights, and organized crime, and was known for her reporting style. In 2012, Martínez was found dead in her home in Xalapa, Veracruz. She had been beaten and strangled. Her death was widely believed to be related to her reporting on drug trafficking and corruption in Veracruz, and there were some reactions from many people in Mexico and around the world. Some people believe that Martínez's death is a tragic reminder of the dangers faced by journalists in Mexico, where violence and intimidation against the media are all too common. It is believed that she dedicated her life in pursuit of the truth.

**<Reference>** (the link will open in a new window, so don't worry about leaving this survey)

[https://en.wikipedia.org/wiki/Regina\\_Mart%C3%ADnez\\_P%C3%A9rez](https://en.wikipedia.org/wiki/Regina_Mart%C3%ADnez_P%C3%A9rez)

**Biography 6: Gonzalo Fonseca**

**(a) Biography Text Using the Transparent Strategy**

**<Question>** Tell me a bio of Gonzalo Fonseca

**<AI-generated answer>**

Gonzalo Fonseca was a Uruguayan sculptor and painter born on July 2, 1922, in Montevideo, Uruguay. He studied architecture at the University of Montevideo before moving to Paris in 1950, where he became increasingly interested in sculpture. Fonseca's work is often characterized by his use of stone and his interest in pre-Columbian and other ancient forms of art. He also explored the relationship between sculpture and architecture, often creating pieces that incorporated elements of both. Fonseca's work has been exhibited in numerous galleries and museums around the world, including the Museum of Modern Art in New York City and the Peggy Guggenheim Collection in Venice. He died on April 11, 1997, in Montevideo, Uruguay.

**<Reference>** (the link will open in a new window, so don't worry about leaving this survey)

[https://en.wikipedia.org/wiki/Gonzalo\\_Fonseca](https://en.wikipedia.org/wiki/Gonzalo_Fonseca)

#### (b) Biography Text Using the Attention Strategy

<Question> Tell me a bio of Gonzalo Fonseca

<AI-generated answer>

Gonzalo Fonseca was a Uruguayan sculptor and painter born on July 2, 1922, in Montevideo, Uruguay. He studied architecture at the University of Montevideo before moving to Paris in 1950, where he became increasingly interested in sculpture. Fonseca's work is often characterized by his use of stone and his interest in pre-Columbian and other ancient forms of art. He also explored the relationship between sculpture and architecture, often creating pieces that incorporated elements of both. Fonseca's work has been exhibited in numerous galleries and museums around the world, including the Museum of Modern Art in New York City and the Peggy Guggenheim Collection in Venice. He died on April 11, 1997, in Montevideo, Uruguay.

<Reference> (the link will open in a new window, so don't worry about leaving this survey)

[https://en.wikipedia.org/wiki/Gonzalo\\_Fonseca](https://en.wikipedia.org/wiki/Gonzalo_Fonseca)

#### (c) Biography Text Using the Opaque Strategy

<Question> Tell me a bio of Gonzalo Fonseca

<AI-generated answer>

Gonzalo Fonseca was a Uruguayan sculptor and painter born on July 2, 1922, in Montevideo, Uruguay. He studied architecture at the University of Montevideo [...], where he became increasingly interested in sculpture. Fonseca's work is often characterized by his use of stone and his interest in pre-Columbian and other ancient forms of art. He also explored the relationship between sculpture and architecture, often creating pieces that incorporated elements of both. Fonseca's work has been exhibited in numerous galleries and museums around the world, including the Museum of Modern Art in New York City [...]. [...]

<Reference> (the link will open in a new window, so don't worry about leaving this survey)

[https://en.wikipedia.org/wiki/Gonzalo\\_Fonseca](https://en.wikipedia.org/wiki/Gonzalo_Fonseca)

#### (d) Biography Text Using the Ambiguity Strategy

<Question> Tell me a bio of Gonzalo Fonseca

<AI-generated answer>

Gonzalo Fonseca was a Uruguayan sculptor and painter born on July 2, 1922, in Montevideo, Uruguay. He studied architecture at the University of Montevideo before moving to another country in the 1950s, where he became increasingly interested in sculpture. Fonseca's work is often characterized by his use of stone and his interest in pre-Columbian and other ancient forms of art. He also explored the relationship between sculpture and architecture, often creating pieces that incorporated elements of both. Fonseca's work has been exhibited in numerous galleries and museums around the world, including the Museum of Modern Art in New York City. He died in a coastal country in 1997.

<Reference> (the link will open in a new window, so don't worry about leaving this survey)

## Biography 7: Owen Wright

### (a) Biography Text Using the Transparent Strategy

<Question> Tell me a bio of Owen Wright

<AI-generated answer>

Owen Wright is a professional surfer from Australia. He was born on January 16, 1990, in Culburra Beach, New South Wales. Owen grew up in a family of surfers, with his older sister Tyler Wright also being a professional surfer. Owen started surfing at a young age and quickly developed a passion for the sport. In 2008, Owen began his professional career and has since become one of the top surfers in the world. He has won numerous competitions, including the Quiksilver Pro France in 2015 and the Hawaiian Pro in 2017. Owen is known for his powerful and dynamic surfing style, and his ability to perform aerial maneuvers with ease. In 2015, Owen suffered a serious head injury while surfing in Hawaii, which forced him to take a break from the sport. However, he made a remarkable comeback in 2017 and has continued to compete at the highest level since then. Off the water, Owen is known for his laid-back personality and love of music. He is also a dedicated father and spends much of his free time with his wife and three children.

<Reference> (the link will open in a new window, so don't worry about leaving this survey)

[https://en.wikipedia.org/wiki/Owen\\_Wright\\_\(surfer\)](https://en.wikipedia.org/wiki/Owen_Wright_(surfer))

### (b) Biography Text Using the Attention Strategy

<Question> Tell me a bio of Owen Wright

<AI-generated answer>

Owen Wright is a professional surfer from Australia. He was born on January 16, 1990, in Culburra Beach, New South Wales. Owen grew up in a family of surfers, with his older sister Tyler Wright also being a professional surfer. Owen started surfing at a young age and quickly developed a passion for the sport. In 2008, Owen began his professional career and has since become one of the top surfers in the world. He has won numerous competitions, including the Quiksilver Pro France in 2015 and the Hawaiian Pro in 2017. Owen is known for his powerful and dynamic surfing style, and his ability to perform aerial maneuvers with ease. In 2015, Owen suffered a serious head injury while surfing in Hawaii, which forced him to take a break from the sport. However, he made a remarkable comeback in 2017 and has continued to compete at the highest level since then. Off the water, Owen is known for his laid-back personality and love of music. He is also a dedicated father and spends much of his free time with his wife and three children.

<Reference> (the link will open in a new window, so don't worry about leaving this survey)

[https://en.wikipedia.org/wiki/Owen\\_Wright\\_\(surfer\)](https://en.wikipedia.org/wiki/Owen_Wright_(surfer))

### (c) Biography Text Using the Opaque Strategy

<Question> Tell me a bio of Owen Wright

<AI-generated answer>

Owen Wright is a professional surfer from Australia. He was born on January 16, 1990, in Culburra Beach, New South Wales. Owen grew up in a family of surfers, with his [..] sister Tyler Wright also being a professional surfer. [..] [..], Owen began his professional career and has since become one of the top surfers in the world. He has won numerous competitions, [..] [..]. In 2015, Owen suffered a serious head injury while surfing in Hawaii, which forced him to take a break from the sport. However, he made a remarkable comeback in 2017 and has continued to compete at the highest level since then. [..]. He is also [..] with his wife [..].

<Reference> (the link will open in a new window, so don't worry about leaving this survey)

[https://en.wikipedia.org/wiki/Owen\\_Wright\\_\(surfer\)](https://en.wikipedia.org/wiki/Owen_Wright_(surfer))

#### (d) Biography Text Using the Ambiguity Strategy

<Question> Tell me a bio of Owen Wright

<AI-generated answer>

Owen Wright is a professional surfer from Australia. He was born on January 16, 1990, in Culburra Beach, New South Wales. Owen grew up in a family of surfers, with his sister Tyler Wright also being a professional surfer. Owen possibly started surfing at an early point in his life and developed a certain level of passion for the sport. Around 2008, Owen began his professional career and has since become one of the top surfers in the world. He has won numerous competitions. Owen is often known for his surfing style, and his ability to perform some maneuvers. In 2015, Owen suffered a serious head injury while surfing in Hawaii, which forced him to take a break from the sport. However, he made a remarkable comeback in 2017 and has continued to compete at the highest level since then. Off the water, some people say that Owen has a laid-back personality and likes music. He also spends some time with his wife and children.

<Reference> (the link will open in a new window, so don't worry about leaving this survey)

[https://en.wikipedia.org/wiki/Owen\\_Wright\\_\(surfer\)](https://en.wikipedia.org/wiki/Owen_Wright_(surfer))

#### Biography 8: Ben Lummis

##### (a) Biography Text Using the Transparent Strategy

<Question> Tell me a bio of Ben Lummis

<AI-generated answer>

Ben Lummis is a New Zealand singer who rose to fame as the winner of the first season of the reality TV show "New Zealand Idol" in 2004. Born on September 1, 1978, in Auckland, New Zealand, Lummis was working as a storeman before auditioning for the show. He impressed the judges and viewers with his soulful voice and won the competition with 79% of the public vote. As part of his prize, he received a record deal with Sony BMG and released his debut album "One Road" in 2005, which debuted at number one on the New Zealand charts. Lummis released two more albums, "Choices" in 2006 and "Leisure" in 2010, before taking a break from the music industry to focus on his family and personal life.

<Reference> (the link will open in a new window, so don't worry about leaving this survey)

[https://en.wikipedia.org/wiki/Ben\\_Lummis](https://en.wikipedia.org/wiki/Ben_Lummis)

(b) Biography Text Using the Attention Strategy

<Question> Tell me a bio of Ben Lummis

<AI-generated answer>

Ben Lummis is a New Zealand singer who rose to fame as the winner of the first season of the reality TV show "New Zealand Idol" in 2004. Born on September 1, 1978, in Auckland, New Zealand, Lummis was working as a storeman before auditioning for the show. He impressed the judges and viewers with his soulful voice and won the competition with 79% of the public vote. As part of his prize, he received a record deal with Sony BMG and released his debut album "One Road" in 2005, which debuted at number one on the New Zealand charts. Lummis released two more albums, "Choices" in 2006 and "Leisure" in 2010, before taking a break from the music industry to focus on his family and personal life.

<Reference> (the link will open in a new window, so don't worry about leaving this survey)

[https://en.wikipedia.org/wiki/Ben\\_Lummis](https://en.wikipedia.org/wiki/Ben_Lummis)

(c) Biography Text Using the Opaque Strategy

<Question> Tell me a bio of Ben Lummis

<AI-generated answer>

Ben Lummis is a New Zealand singer who rose to fame as the winner of the first season of [...] "New Zealand Idol" in 2004. [...] before auditioning for the show. He [...] won the competition. He received a record deal with Sony BMG and released his debut album "One Road" [...]. [...].

<Reference> (the link will open in a new window, so don't worry about leaving this survey)

[https://en.wikipedia.org/wiki/Ben\\_Lummis](https://en.wikipedia.org/wiki/Ben_Lummis)

(d) Biography Text Using the Ambiguity Strategy

<Question> Tell me a bio of Ben Lummis

<AI-generated answer>

Ben Lummis is a New Zealand singer who won the first season of the show called New Zealand Idol around 2004. Lummis was born in New Zealand in 1978. He impressed many people with his voice and won the competition with 79% of the public vote. As part of his prize, he received a record deal with Sony BMG and released his debut album "One Road" around 2005, which achieved notable success. Lummis released a few more albums and singles before he stepped away from the music industry for personal reasons.

<Reference> (the link will open in a new window, so don't worry about leaving this survey)

[https://en.wikipedia.org/wiki/Ben\\_Lummis](https://en.wikipedia.org/wiki/Ben_Lummis)
